# Supplementary material for: The inverse Kalman filter
Source: arXiv:2407.10089 ancillary file (2026-07-10)
Supplement: Supplementary file 1 [file IKF_arXiv_SI.pdf]

# Supplementary material for "The inverse Kalman filter"

Xinyi Fang and Mengyang Gu

**Abstract**

This file provides supplementary information for "The inverse Kalman filter." It includes proofs for all lemmas and establishes the relationship between Gaussian processes with Matérn covariance functions and dynamic linear models. It describes the conjugate gradient algorithm and outlines procedures for scalable computation of the predictive distribution in particle dynamics. It also demonstrates the application of the IKF-CG algorithm for predicting missing values in lattice data. Additionally, it introduces parameter estimation approaches of both applications, analyzes the corresponding computational complexity, and provides additional numerical results for particle interactions and missing value predictions.

## S1 Proofs

In the following proofs, we first prove Lemma A2 and Lemma 2, as these lemmas are essential for proving Lemma 3. The outcome of Lemma 3 is then used to prove Lemma 1. The proof of Lemma 4 is presented at the end.

*Proof of Lemma A2.* From (A2) in step (ii) of the Kalman filter in Lemma A1, we have

$$p(\mathbf{y}_{1:N}) = \prod_{t=1}^{N} \left\{ (2\pi Q_t)^{-\frac{1}{2}} \exp\left( -\frac{(y_t - f_t)^2}{2Q_t} \right) \right\}. \tag{S1}$$

Additionally, since $\mathbf{y}_{1:N}$ follows a zero-mean multivariate normal distribution, we have

$$p(\mathbf{y}_{1:N}) = (2\pi)^{-\frac{N}{2}} |\boldsymbol{\Sigma}|^{-\frac{1}{2}} \exp\left( -\frac{1}{2} (\mathbf{L}^{-1}\mathbf{y})^T (\mathbf{L}^{-1}\mathbf{y}) \right), \tag{S2}$$

where $\mathbf{L}$ is the Cholesky factor of $\boldsymbol{\Sigma}$, a lower triangular matrix with positive diagonal entries. By equating (S1) and (S2), we have

$$\sum_{t=1}^{N} \frac{(y_t - f_t)^2}{Q_t} = (\mathbf{L}^{-1}\mathbf{y})^T (\mathbf{L}^{-1}\mathbf{y}) = \sum_{t=1}^{N} \tilde{y}_t^2, \tag{S3}$$

$$\prod_{t=1}^{N} Q_t^{\frac{1}{2}} = |\boldsymbol{\Sigma}|^{\frac{1}{2}} = |\mathbf{L}| = \prod_{t=1}^{N} L_{t,t}. \tag{S4}$$

Since the Kalman filter operates incrementally and applies to any number of observations, these equalities hold not only for the entire set of observations up to $N$ but also for any subset up to $t' \leqslant N$. This means the expressions in (S3) and (S4) are valid for sums and products up to any $t' = 1, ..., N$. We will use this property to prove both statements of the lemma by mathematical induction.

First, we prove $\tilde{y}_t = (y_t - f_t)/Q_t^{1/2}$ for $t = 1, ..., N$. When we consider only the first observation, i.e., $t' = 1$, the matrix $\boldsymbol{\Sigma}$ reduces to the scalar $Q_1$, and the statement directly follows from the

definition of the Cholesky decomposition which has positive diagonals and $f_1 = 0$. For the first $t' - 1$ observations, we have $\sum_{t=1}^{t'-1}(y_t - f_t)^2/Q_t = \sum_{t=1}^{t'-1} \tilde{y}_t^2$. Including the $t'$th observation, we get $\sum_{t=1}^{t'}(y_t - f_t)^2/Q_t = \sum_{t=1}^{t'} \tilde{y}_t^2$. Subtracting the sum of the first $t' - 1$ observations, we have $(y_{t'} - f_{t'})^2/Q_{t'} = \tilde{y}_{t'}^2$, which gives

$$\tilde{y}_{t'} = \frac{y_{t'} - f_{t'}}{Q_{t'}^{1/2}} \qquad \text{or} \qquad \tilde{y}_{t'} = -\frac{(y_{t'} - f_{t'})}{Q_{t'}^{1/2}}, \tag{S5}$$

where $f_{t'}$ is not related to the observation $y_{t'}$ based on the Kalman filter. Let $\tilde{L}_{t',t}$ denote the $(t', t)$th element of $\mathbf{L}^{-1}$. We can write

$$\tilde{y}_{t'} = \sum_{t=1}^{t'} \tilde{L}_{t',t} y_t. \tag{S6}$$

By equating the coefficient of $y_{t'}$ in (S5) and (S6), we obtain $\tilde{L}_{t',t'} = Q_{t'}^{-1/2}$ or $\tilde{L}_{t',t'} = -Q_{t'}^{-1/2}$. As $\mathbf{L}^{-1}\mathbf{L} = \mathbf{I}_N$ and $\mathbf{L}$ is a lower triangular matrix with the diagonal value $L_{t',t'} > 0$ for $t' = 1, ..., N$, then $\tilde{L}_{t',t'} = 1/L_{t',t'} > 0$. The only solution is $\tilde{y}_{t'} = (y_{t'} - f_{t'})/Q_{t'}^{1/2}$.

The second statement, $L_{t,t} = Q_t^{1/2}$, follows the similar logic with (S4) by mathematical induction. The detailed proof is omitted here for brevity. □

*Proof of Lemma 2.* For any $t = 1, ..., N$, we invert (A4) in Kalman filter to compute $x_t = f_t + Q_t^{1/2} \tilde{x}_t$ with $f_t = \mathbf{F}_t \mathbf{b}_t$, which leads to (8). The other two steps in (7)-(9) are from the Kalman filter with a known observation $x_t$. By Lemma A2, for any N-vector $\mathbf{x}$, the second step of Kalman filter produces $\tilde{\mathbf{x}} = \mathbf{L}^{-1}\mathbf{x}$. As the steps of Kalman filter are reversed in Lemma 2, we have $\mathbf{x} = \mathbf{L}\tilde{\mathbf{x}}$ for any N-vector $\tilde{\mathbf{x}}$. □

*Proof of Lemma 3.* Denote $\mathbf{x} = \mathbf{L}\tilde{\mathbf{x}}$. The $t'$th entry $x_{t'}$ is

$$x_{t'} = \sum_{t=1}^{t'} L_{t',t} \tilde{x}_t. \tag{S7}$$

We will prove (10) with $\ell_{t,t'}$ defined in (11) using the mathematical induction. By Lemma A2, we have $L_{t',t} = Q_t^{1/2}$ for $t' = t$, so $L_{1,1} = Q_1^{1/2}$. First, we show that $L_{t',t'-1} = Q_{t'-1}^{1/2} \ell_{t',t'-1}$. For $x_{t'}$, we iterate through equations in Lemma 2 to get

$$x_{t'} = \mathbf{F}_{t'} \mathbf{G}_{t'} (\mathbf{b}_{t'-1} + \mathbf{K}_{t'-1} Q_{t'-1}^{\frac{1}{2}} \tilde{x}_{t'-1}) + Q_{t'}^{\frac{1}{2}} \tilde{x}_{t'}. \tag{S8}$$

Note that $\mathbf{b}_{t'-1}$ does not depend on $\tilde{x}_{t'-1}$ or $\tilde{x}_{t'}$. From (S7) and Lemma A2, we also have

$$x_{t'} = \sum_{t=1}^{t'-2} L_{t',t} \tilde{x}_t + L_{t',t'-1} \tilde{x}_{t'-1} + Q_{t'}^{\frac{1}{2}} \tilde{x}_{t'}. \tag{S9}$$

By equating (S8) and (S9), we obtain that for $t' = t + 1$, $L_{t',t} = L_{t',t'-1} = \mathbf{F}_{t'} \mathbf{G}_{t'} \mathbf{K}_{t'-1} Q_{t'-1}^{1/2} = Q_t^{1/2} \ell_{t',t}$, where $\ell_{t',t} = \mathbf{F}_{t'} \mathbf{G}_{t'} \mathbf{K}_{t'-1}$.

Now, assume that for any $t' \geqslant t + 1$, $L_{t',t} = Q_t^{1/2} \ell_{t',t} = Q_t^{1/2} \mathbf{F}_{t'} \left( \prod_{l=t+1}^{t'} \mathbf{G}_l \right) \mathbf{K}_t$. We will show that this result holds for $L_{t'+1,t}$. From (S7), Lemma A2 and plugging $L_{t',t} = Q_t^{1/2} \ell_{t',t} =$

$Q_t^{1/2}\mathbf{F}_{t'}\left(\prod_{l=t+1}^{t'}\mathbf{G}_l\right)\mathbf{K}_t$ for $t'\geqslant t+1$, we have

$$x_{t'} = \mathbf{F}_{t'}\sum_{t=1}^{t'-1} Q_t^{\frac{1}{2}}\left(\prod_{l=t+1}^{t'}\mathbf{G}_l\right)\mathbf{K}_t\tilde{x}_t + Q_{t'}^{\frac{1}{2}}\tilde{x}_{t'}. \tag{S10}$$

Compare (S10) with (8) in Lemma 2, we obtain $\mathbf{b}_{t'} = \sum_{t=1}^{t'-1} Q_t^{1/2}\left(\prod_{l=t+1}^{t'}\mathbf{G}_l\right)\mathbf{K}_t\tilde{x}_t$. Then iterate through Lemma 2, we derive

$$\begin{aligned}
\mathbf{m}_{t'} &= \sum_{t=1}^{t'-1} Q_t^{\frac{1}{2}}\left(\prod_{l=t+1}^{t'}\mathbf{G}_l\right)\mathbf{K}_t\tilde{x}_t + \mathbf{K}_{t'}Q_{t'}^{\frac{1}{2}}\tilde{x}_{t'},\\
\mathbf{b}_{t'+1} &= \sum_{t=1}^{t'-1} Q_t^{\frac{1}{2}}\left(\prod_{l=t+1}^{t'+1}\mathbf{G}_l\right)\mathbf{K}_t\tilde{x}_t + \mathbf{G}_{t'+1}\mathbf{K}_{t'}Q_{t'}^{\frac{1}{2}}\tilde{x}_{t'},\\
x_{t'+1} &= \mathbf{F}_{t'+1}\left(\sum_{t=1}^{t'-1} Q_t^{\frac{1}{2}}\left(\prod_{l=t+1}^{t'+1}\mathbf{G}_l\right)\mathbf{K}_t\tilde{x}_t + \mathbf{G}_{t'+1}\mathbf{K}_{t'}Q_{t'}^{\frac{1}{2}}\tilde{x}_{t'}\right) + Q_{t'+1}^{\frac{1}{2}}\tilde{x}_{t'+1},\\
&= \mathbf{F}_{t'+1}\left(\sum_{t=1}^{t'} Q_t^{\frac{1}{2}}\left(\prod_{l=t+1}^{t'+1}\mathbf{G}_l\right)\mathbf{K}_t\tilde{x}_t\right) + Q_{t'+1}^{\frac{1}{2}}\tilde{x}_{t'+1}.
\end{aligned} \tag{S11}$$

By equating (S11) with (S7) for $x_{t'+1}$: $x_{t'+1} = \sum_{t=1}^{t'} L_{t'+1,t}\tilde{x}_t + L_{t'+1,t'+1}\tilde{x}_{t'+1}$, we get $L_{t'+1,t} = Q_t^{1/2}\mathbf{F}_{t'+1}\left(\prod_{l=t+1}^{t'+1}\mathbf{G}_l\right)\mathbf{K}_t = Q_t^{1/2}\ell_{t'+1,t}$, thus completing the proof. □

*Proof of Lemma 1.* Denote $\tilde{\mathbf{x}} = \mathbf{L}^T\mathbf{u}$. The $N$th and $(N-1)$th entries of $\tilde{\mathbf{x}}$ directly follow from Lemma 3. For $t = N-2,\ldots,1$, we will prove by induction. For the $t$th entry $x_t$, by Lemma 3, we have

$$\tilde{x}_t = \sum_{t'=t}^{N} L_{t',t}u_{t'} = Q_t^{\frac{1}{2}}\left(\sum_{t'=t+2}^{N}\ell_{t',t}u_{t'} + \ell_{t+1,t}u_{t+1} + u_t\right).$$

Thus, it suffices to prove $\tilde{\ell}_{t+1,t} = \mathbf{g}_{t+1}\mathbf{G}_{t+1}\mathbf{K}_t = \sum_{t'=t+2}^{N}\ell_{t',t}u_{t'}$. When $t = N-2$,

$$\ell_{N,N-2}u_N = \mathbf{F}_N\mathbf{G}_N\mathbf{G}_{N-1}\mathbf{K}_{N-2}u_N = \mathbf{g}_{N-1}\mathbf{G}_{N-1}\mathbf{K}_{N-2} = \tilde{\ell}_{N-1,N-2}.$$

Assume for any given $t$ with $t \leqslant N-2$, $\mathbf{g}_{t+1}\mathbf{G}_{t+1}\mathbf{K}_t = \sum_{t'=t+2}^{N}\ell_{t',t}u_{t'}$. We will prove the formula holds for $t-1$. From Lemma 3, we have

$$\sum_{t'=t+2}^{N}\ell_{t',t}u_{t'} = \sum_{t'=t+2}^{N}\mathbf{F}_{t'}\left(\prod_{l=t+1}^{t'}\mathbf{G}_l\right)\mathbf{K}_t u_{t'} = \left\{\sum_{t'=t+2}^{N}\mathbf{F}_{t'}\left(\prod_{l=t+2}^{t'}\mathbf{G}_l\right)u_{t'}\right\}\mathbf{G}_{t+1}\mathbf{K}_t,$$

where the last equation hols as $u_{t'}$ is a scalar. Thus

$$\mathbf{g}_{t+1} = \sum_{t'=t+2}^{N}\mathbf{F}_{t'}\left(\prod_{l=t+2}^{t'}\mathbf{G}_l\right)u_{t'}.$$

Then for $(t-1)$th entry, similarly we have

$$\begin{aligned}\sum_{t'=t+1}^{N} \ell_{t',t-1} u_{t'} &= \left\{ \sum_{t'=t+1}^{N} \mathbf{F}_{t'} \left( \prod_{l=t+1}^{t'} \mathbf{G}_l \right) u_{t'} \right\} \mathbf{G}_t \mathbf{K}_{t-1} \\ &= \{\mathbf{g}_{t+1}\mathbf{G}_{t+1} + \mathbf{F}_{t+1}\mathbf{G}_{t+1}u_{t+1}\} \mathbf{G}_t \mathbf{K}_{t-1} \\ &= \mathbf{g}_t \mathbf{G}_t \mathbf{K}_{t-1},\end{aligned}$$

where the last equation follows from (5). Therefore, $\mathbf{g}_t\mathbf{G}_t\mathbf{K}_{t-1} = \sum_{t'=t+1}^{N} \ell_{t',t-1}u_{t'}$ and we have proved the results hold for $t-1$ from any given $t \leqslant N-1$ which concludes the proof. □

*Proof of Lemma 4.* In Lemma 1, the iterative algorithm gives $\tilde{\mathbf{x}} = \mathbf{L}^T\mathbf{u}$ for any N-vector $\mathbf{u}$. We invert (4) to get $u_t = Q_t^{-1/2}\tilde{x}_t - \tilde{\ell}_{t+1,t} - \ell_{t+1,t}u_{t+1}$ for any $t$, which leads to (12). Since we reverse the steps of the iterative algorithm in Lemma 1, we have $\mathbf{u} = (\mathbf{L}^T)^{-1}\tilde{\mathbf{x}}$ for any N-vector $\tilde{\mathbf{x}}$. □

## S2 Gaussian processes with half-integer Matérn covariances as dynamic linear models

In this section, we provide the connection between Gaussian processes having the Matérn covariance with roughness parameters $\nu = 1/2$ and $\nu = 5/2$ and dynamic linear models (DLMs). Let $y_t = y(d_t)$ for $t = 1, ..., N$, modeled as

$$y(d_t) = z(d_t) + v_t,$$

with $z(\cdot)$ follows a zero-mean Gaussian process with covariance function $c(\cdot,\cdot)$ and range parameter $\gamma$, and $v_t$ represents independent Gaussian noise with variance $V_t$.

For a Gaussian process having Matérn covariance function with roughness parameter $\nu = 2.5$ in (15), the latent stochastic process $z(\cdot)$ can be expressed via stochastic differential equations [12]:

$$\dot{\boldsymbol{\theta}}(d) = \mathbf{J}\boldsymbol{\theta}(d) + \tilde{\mathbf{F}}u(d), \tag{S12}$$

or equivalently in matrix form

$$\frac{\partial}{\partial d}\begin{pmatrix} z(d) \\ z^{(1)}(d) \\ z^{(2)}(d) \end{pmatrix} = \begin{pmatrix} 0 & 1 & 0 \\ 0 & 0 & 1 \\ -\lambda^3 & -3\lambda^2 & -3\lambda \end{pmatrix} \begin{pmatrix} z(d) \\ z^{(1)}(d) \\ z^{(2)}(d) \end{pmatrix} + \begin{pmatrix} 0 \\ 0 \\ 1 \end{pmatrix} u(d),$$

where $\partial$ denotes the differentiation, $z^{(p)}(\cdot)$ denotes the $p$th derivative of the process $z(\cdot)$, and $u(d) \sim \mathcal{N}(0, \sigma^2)$ follows Gaussian white noise with variance $\sigma^2$, $\lambda = \sqrt{2\nu}/\gamma$.

For any $d_t$ with $t = 1, ..., N$, the solution of (S12) can be represented as a DLM:

$$y(d_t) = \mathbf{F}\boldsymbol{\theta}(d_t) + v_t, \tag{S13}$$

$$\boldsymbol{\theta}(d_t) = \mathbf{G}(d_t)\boldsymbol{\theta}(d_{t-1}) + \mathbf{w}(d_t),\ \mathbf{w}(d_t) \sim \mathcal{MN}(\mathbf{0}, \mathbf{W}(d_t)), \tag{S14}$$

where $\mathbf{G}(d_t) = e^{\mathbf{J}(d_t - d_{t-1})}$, $\mathbf{W}(d_t) = \int_0^{d_t - d_{t-1}} e^{\mathbf{J}s}\tilde{\mathbf{F}}q\tilde{\mathbf{F}}^T e^{\mathbf{J}^T s} ds$ for $t = 2, \ldots, N$, $\mathbf{F} = [1, 0, 0]$, and the stationary distribution is $\boldsymbol{\theta}(d_t) \sim \mathcal{MN}(\mathbf{0}, \mathbf{W}(d_1))$ with $\mathbf{W}(d_1) = \int_0^{\infty} e^{\mathbf{J}s}\tilde{\mathbf{F}}q\tilde{\mathbf{F}}^T e^{\mathbf{J}^T s} ds$.

Write $\mathbf{G}(d_t) = \mathbf{G}_t$, $\mathbf{W}(d_t) = \mathbf{W}_t$ and $\boldsymbol{\theta}(d_t) = \boldsymbol{\theta}_t$, the joint distribution of $(\boldsymbol{\theta}_1^T, \ldots, \boldsymbol{\theta}_N^T)^T$ follows a multivariate normal distribution with the covariance being the inverse of a block tri-diagonal matrix

$$\begin{pmatrix} \boldsymbol{\theta}_1 \\ \boldsymbol{\theta}_2 \\ \boldsymbol{\theta}_3 \\ \vdots \\ \boldsymbol{\theta}_N \end{pmatrix} \sim \mathcal{MN}\left(\mathbf{0}, \begin{pmatrix} \boldsymbol{W}_1^{-1} + \boldsymbol{G}_2^T \boldsymbol{W}_2^{-1} \boldsymbol{G}_2 & -\boldsymbol{G}_2^T \boldsymbol{W}_2^{-1} & & & \\ -\boldsymbol{W}_2^{-1} \boldsymbol{G}_2 & \boldsymbol{W}_2^{-1} + \boldsymbol{G}_3^T \boldsymbol{W}_3^{-1} \boldsymbol{G}_3 & & & \\ & \ddots & \ddots & \ddots & \\ & & & \boldsymbol{W}_{N-1}^{-1} + \boldsymbol{G}_N^T \boldsymbol{W}_N^{-1} \boldsymbol{G}_N & -\boldsymbol{G}_{N-1}^T \boldsymbol{W}_{N-1}^{-1} \\ & & & -\boldsymbol{W}_{N-1}^{-1} \boldsymbol{G}_{N-1} & \boldsymbol{W}_N^{-1} \end{pmatrix}^{-1}\right), \tag{S15}$$

where all $\mathbf{G}_t$ and $\mathbf{W}_t$ have closed-form expressions as a function of $\Delta_t = |d_t - d_{t-1}|$ and $\lambda = \sqrt{2\nu}/\gamma$:

$$\mathbf{G}_t = e^{\mathbf{J}\Delta_t} = \frac{e^{-\lambda\Delta_t}}{2} \begin{pmatrix} \lambda^2\Delta_t^2 + 2\lambda + 2 & 2(\lambda\Delta_t^2 + \Delta_t) & \Delta_t^2 \\ -\lambda^3\Delta_t^2 & -2(\lambda^2\Delta_t^2 - \lambda\Delta_t - 1) & 2\Delta_t - \lambda\Delta_t^2 \\ \lambda^4\Delta_t^2 - 2\lambda^3\Delta_t & 2(\lambda^3\Delta_t^2 - 3\lambda^2\Delta_t) & \lambda^2\Delta_t^2 - 4\lambda\Delta_t + 2 \end{pmatrix}$$

$$\mathbf{W}(d_t) = \frac{4\sigma^2\lambda^5}{3} \begin{pmatrix} W_{1,1}(d_t) & W_{1,2}(d_t) & W_{1,3}(d_t) \\ W_{2,1}(d_t) & W_{2,2}(d_t) & W_{2,3}(d_t) \\ W_{3,1}(d_t) & W_{3,2}(d_t) & W_{3,3}(d_t) \end{pmatrix},$$

$$\begin{aligned}
W_{1,1}(d_t) &= \frac{e^{-2\lambda\Delta_t}(3 + 6\lambda\Delta_t + 6\lambda^2\Delta_t^2 + 4\lambda^3\Delta_t^3 + 2\lambda^4\Delta_t^4) - 3}{-4\lambda^5}, \\
W_{1,2}(d_t) &= W_{2,1}(d_t) = \frac{e^{-2\lambda\Delta_t}\Delta_t^4}{2}, \\
W_{1,3}(d_t) &= W_{3,1}(d_t) = \frac{e^{-2\lambda\Delta_t}(1 + 2\lambda\Delta_t + 2\lambda^2\Delta_t^2 + 4\lambda^3\Delta_t^3 - 2\lambda^4\Delta_t^4) - 1}{4\lambda^3}, \\
W_{2,2}(d_t) &= \frac{e^{-2\lambda\Delta_t}(1 + 2\lambda\Delta_t + 2\lambda^2\Delta_t^2 - 4\lambda^3\Delta_t^3 + 2\lambda^4\Delta_t^4) - 1}{-4\lambda^3}, \\
W_{2,3}(d_t) &= W_{3,2}(d_t) = \frac{e^{-2\lambda\Delta_t}\Delta_t^2(4 - 4\lambda\Delta_t + \lambda^2\Delta_t^2)}{2}, \\
W_{3,3}(d_t) &= \frac{e^{-2\lambda\Delta_t}(-3 + 10\lambda\Delta_t - 22\lambda^2\Delta_t^2 + 12\lambda^3\Delta_t^3 - 2\lambda^4\Delta_t^4) + 3}{4\lambda},
\end{aligned}$$

and

$$\mathbf{W}(d_1) = \begin{pmatrix} \sigma^2 & 0 & -\sigma^2\lambda^2/3 \\ 0 & \sigma^2\lambda^2/3 & 0 \\ -\sigma^2\lambda^2/3 & 0 & \sigma^2\lambda^4 \end{pmatrix}.$$

For Gaussian processes with exponential covariance functions or, equivalently, the Matérn covariance functions with the roughness parameter being $\nu = 1/2$, the corresponding DLM representation follows (S13)-(S14) with $F_t = 1$, $G_t = \exp(-|d_t - d_{t-1}|/\gamma)$ and $W_t = \sigma^2(1 - G_t)$ for $t = 2, ..., N$. The stationary distribution $z(d_t) \sim \mathcal{N}(0, \sigma^2)$. The joint distribution $(y_1, ..., y_N)^T$ follows (S15), where the inverse covariance matrix is a tri-diagonal matrix. All results shown above are coded in the `FastGaSP` package on CRAN [9].

# S3 The conjugate gradient method

The conjugate gradient (CG) algorithm [13] is an iterative method to solve a linear system $\mathbf{\Sigma}_y\hat{\mathbf{u}} = \mathbf{y}$, particularly useful for a sparse matrix $\mathbf{\Sigma}_y$. The key advantage of the conjugate gradient

**Algorithm S1** Conjugate gradient algorithm

**Input:** $\mathbf{\Sigma}_y$, $\mathbf{y}$ from the linear system $\mathbf{\Sigma}_y\hat{\mathbf{u}} = \mathbf{y}$, maximum iteration $i_{max}$, and the error tolerance $tol$.

$i \leftarrow 0$
$\hat{\mathbf{u}} \leftarrow \mathbf{0}$
$\boldsymbol{\varepsilon} \leftarrow \mathbf{y} - \mathbf{\Sigma}_y\hat{\mathbf{u}}$
$\mathbf{u} \leftarrow \boldsymbol{\varepsilon}$
$\delta_{old} \leftarrow \boldsymbol{\varepsilon}^T\boldsymbol{\varepsilon}$
$\delta_{new} \leftarrow 1$
**while** $i < i_{max}$ and $\delta_{new} > tol$ **do**
    $\tilde{\mathbf{u}} \leftarrow \mathbf{\Sigma}_y\mathbf{u}$
    $\alpha \leftarrow \delta_{old}/(\mathbf{u}^T\tilde{\mathbf{u}})$
    $\hat{\mathbf{u}} \leftarrow \hat{\mathbf{u}} + \alpha\mathbf{u}$
    $\boldsymbol{\varepsilon} \leftarrow \boldsymbol{\varepsilon} - \alpha\tilde{\mathbf{u}}$
    $\delta_{new} \leftarrow \boldsymbol{\varepsilon}^T\boldsymbol{\varepsilon}$
    $\delta_{ratio} \leftarrow \delta_{new}/\delta_{old}$
    $\mathbf{u} \leftarrow \boldsymbol{\varepsilon} + \delta_{ratio}\mathbf{u}$
    $\delta_{old} \leftarrow \delta_{new}$
    $i \leftarrow i + 1$
**end while**

**Output:** $\hat{\mathbf{u}}$.

algorithm is that it avoids the computationally intensive matrix inversion and only requires matrix-vector multiplication, making it a potentially scalable alternative for large-scale applications. The detailed algorithm is summarized in Algorithm S1.

## S4 Scalable computation of the predictive distribution in particle dynamics

In this section, we detail the scalable computation of the predictive mean and variance for the particle interaction function in (18) and (19), respectively, applicable to both single and multiple test inputs. We use an example of particles on 2-dimensional spatial coordinates to illustrate the data pre-processing step. The space is divided into $n_1 \times n_2$ grids, where $n_1$ and $n_2$ represent the number of grids along the two orthogonal coordinates. Each particle is assigned to a grid, with neighboring particles located within the adjacent nine grids, as depicted in Fig. S1(a). For each grid, we record the positions and velocities of particles within the adjacent nine grids. This step is critical as it allows efficient neighbor searching within the adjacent grids during parameter estimation, avoiding the need to loop over all particles. The computational cost of this step is $\mathcal{O}(\sum_{\tau=1}^{n_\tau} n_p(\tau))$, where $n_p(\tau)$ is the number of particles at time $\tau$, and it needs to be performed only once. Following the pre-processing step, constructing neighboring distances for each type of interaction incurs $\mathcal{O}(p_j \sum_{\tau=1}^{n_\tau} n_p(\tau))$ operations, with $p_j$ being the average number of particles in the neighboring nine grids for $j$th interaction, typically no larger than 10 in our applications, which is much smaller than $n_p(\tau)$, thereby reducing the cost substantially compared to $\mathcal{O}(\sum_{\tau=1}^{n_\tau}(n_p(\tau))^2)$ without the pre-processing step.

For prediction on either single or multiple test inputs, the primary computational task is solving for $\hat{\mathbf{u}} = \mathbf{\Sigma}_y^{-1}\mathbf{y}$, where $\mathbf{y}$ is a vector of $\tilde{N}$ dimensions. This is equivalent to solving a linear system

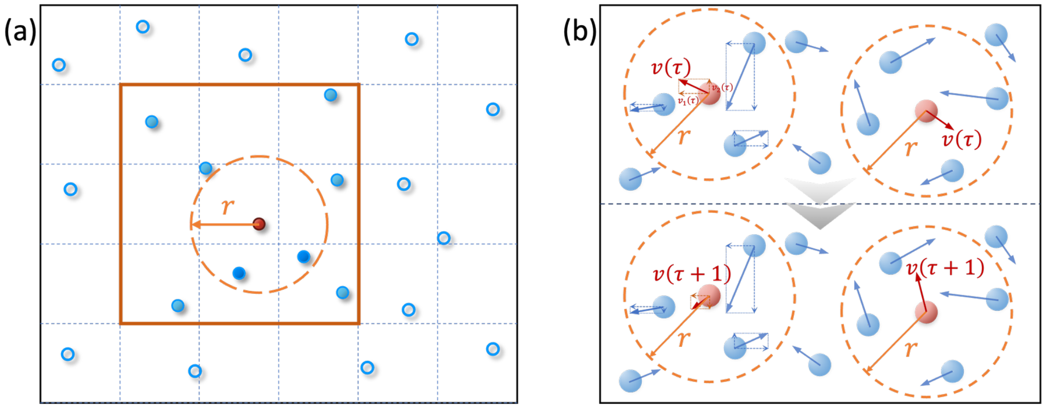


Figure S1: (a) Illustration for preprocessing the particles into coarse-grained grids. The domain is divided into square grid cells with side lengths equal to or greater than the maximum interaction radius. For a given particle (red dot), as only particles in the current and eight adjacent grid cells (orange square region) need to be considered, it substantially accelerates the computation. Particles (blue dots) within the interaction radius (the dashed circle) and itself (red dot) can be identified as neighbors. (b) Visualization of velocity alignment in the unnormalized Vicsek model. Each red particle updates its velocity $v(\tau) = [v_1(\tau), v_2(\tau)]^T$ by aligning with all neighboring particles, including itself, within interaction radius $r$. While all particles simultaneously update their directions, this illustration focuses on the movement of the red particle.

$\mathbf{\Sigma}_y \hat{\mathbf{u}} = \mathbf{y}$, which can be computed iteratively by the conjugate gradient algorithm. Starting with an initial guess $\mathbf{u}_{(0)} = \mathbf{0}$, the conjugate gradient method iteratively refines the solution $\mathbf{u}_{(k)}$ within the Krylov subspace span$[\mathbf{y}, \mathbf{\Sigma}_y\mathbf{y}, \ldots, \mathbf{\Sigma}_y^{k-1}\mathbf{y}]$ at each step $k$, minimizing the norm $||\hat{\mathbf{u}} - \mathbf{u}_{(k)}||^2_{\Sigma_y} = (\hat{\mathbf{u}} - \mathbf{u}_{(k)})^T \mathbf{\Sigma}_y (\mathbf{u} - \mathbf{u}_{(k)})$. In each iteration step, we need to compute $\mathbf{\Sigma}_y \mathbf{u} = (\sum_{j=1}^J \mathbf{A}_j \mathbf{\Sigma}_j^{(u)} \mathbf{A}_j^T + \sigma_0^2 \mathbf{I}_{\tilde{N}})\mathbf{u}$ for any $\tilde{N}$-dimensional vector $\mathbf{u}$, as detailed in Algorithm S1 in Section S3. For each interaction $j, j = 1, \ldots, J$, we decompose the computation of $\mathbf{A}_j \mathbf{\Sigma}_j^{(u)} \mathbf{A}_j^T \mathbf{u}$ into four steps.

In Step 1, we compute $\mathbf{u}_j^{(u)} = \mathbf{A}_j^T \mathbf{u}$, where $\mathbf{A}_j$ is a sparse block diagonal matrix of dimensions $\tilde{N} \times N_j$, with the $i$th digonal block being $\mathbf{A}_{i,j} = [\mathbf{a}_{i,j,1}, \ldots, \mathbf{a}_{i,j,p_{i,j}}]$ for $i = 1, \ldots, n$. We stack all non-zero terms in $\mathbf{A}_j$ as a vector $\mathbf{a}_j = [\text{vec}(\mathbf{A}_{1,j})^T, \ldots, \text{vec}(\mathbf{A}_{n,j})^T]^T = [\text{vec}(\mathbf{a}_{1,j})^T, \ldots, \text{vec}(\mathbf{a}_{N_j,j})^T]^T$ of dimension $D_y N_j$, where vec$(\cdot)$ denotes the vectorization operation and $\mathbf{a}_{t,j} = \mathbf{a}_{i,j,k}$ with $t = \sum_{i'=1}^{i} p_{i',j} + k$ for $i = 1, \ldots, n$ and $k = 1, \ldots, p_{i,j}$, with $p_{0,j} = 0$. The $t$th entry of $\mathbf{u}_j^{(u)}$, denoted as $u_{t,j}^{(u)}$, can be computed by

$$u_{t,j}^{(u)} = \mathbf{a}_{t,j}^T \mathbf{u}_{(t-1)D_y + (1:D_y)},$$

where $\mathbf{u}_{(t-1)D_y+(1:D_y)}$ is a vector containing the $((t-1)D_y + 1)$th to $tD_y$th entries of $\mathbf{u}$.

In Step 2, we rearrange $\mathbf{u}_j^{(u)}$ into $\mathbf{u}_j$ based on the sorted order from $\mathbf{d}_j^{(u)} = [d_{1,j}^{(u)}, \ldots, d_{N_j,j}^{(u)}]^T$ to $\mathbf{d}_j = [d_{1,j}, \ldots, d_{N_j,j}]^T$. We obtain the index set $\{g_t\}_{t=1}^{N_j}$, where $d_{g_t,j}^{(u)} = d_{t,j}$. Using this index set, the $t$th entry of $\mathbf{u}_j$ is $u_{t,j} = u_{g_t,j}^{(u)}$.

In Step 3, we use the IKF algorithm presented in Algorithm 1 to compute $\mathbf{x}_j = \mathbf{\Sigma}_j \mathbf{u}_j$. We then rearrange the entries of $\mathbf{x}_j$ from $\mathbf{x}_j = [x_{1,j}, \ldots, x_{N_j,j}]^T$ to $\mathbf{x}_j^{(u)} = [x_{1,j}^{(u)}, \ldots, x_{N_j,j}^{(u)}]^T$, where $x_{g_t,j}^{(u)} = x_{t,j}$, to preserve the original order of $\mathbf{u}_j$ for subsequent calculations.

In Step 4, we compute $\hat{\mathbf{u}}_j = \mathbf{A}_j \mathbf{x}_j^{(u)}$. We partition the vector $\hat{\mathbf{u}}_j$ into $\hat{\mathbf{u}}_j = [\hat{\mathbf{u}}_{1,j}^T, \ldots, \hat{\mathbf{u}}_{n,j}^T]$, where

each sub-vector $\hat{\mathbf{u}}_{i,j}$ has $D_y$ dimensions and can be computed by

$$\hat{\mathbf{u}}_{i,j} = \mathbf{A}_{i,j}\mathbf{x}^{(u)}_{i,j},$$

with $\mathbf{x}^{(u)}_{i,j}$ being the $(\sum_{i'=1}^{i-1} p_{i',j} + (1 : p_{i,j}))$th entry of the vector $\mathbf{x}^{(u)}_j$ for $i = 1, \ldots, n$.

After completing these four steps for $j = 1, .., J$, we obtain $\mathbf{\Sigma}_y\mathbf{u} = \sum_{j=1}^{J} \hat{\mathbf{u}}_j + \sigma_0^2\mathbf{u}$. These steps are repeated iteratively in a conjugate gradient algorithm to compute $\hat{\mathbf{u}} = \mathbf{\Sigma}_y^{-1}\mathbf{y}$.

The output of the conjugate gradient algorithm, $\hat{\mathbf{u}}$, is used to calculate the predictive mean. We will first explain how to compute the predictive mean and variance for a single test input, and then discuss a scalable approach to compute the predictive mean of a latent interaction function on a large number of inputs. In both scenarios, we first compute the matrix-vector multiplication $\hat{\mathbf{u}}_j = \mathbf{A}_j^T\hat{\mathbf{u}}$ using Step 1 above.

The process of calculating the predictive distribution for a single test input distance $d^*$ is straightforward. Once $N_j$-vector $\mathbf{\Sigma}^{(u)}_j(d^*)$ is constructed, the predictive mean can be obtained by direct vector-matrix multiplication: $\hat{z}_j(d^*) = \mathbf{\Sigma}^{(u)}_j(d^*)^T\hat{\mathbf{u}}_j$. To compute the predictive variance in (19), we first calculate the $N_j$-dimensional vector $\tilde{\mathbf{\Sigma}}^{(u)}_j(d^*) = \mathbf{A}_j\mathbf{\Sigma}^{(u)}_j(d^*)$ using Step 1. Then Steps 1-4 in the conjugate gradient algorithm are applied to compute $\hat{\mathbf{\Sigma}}^{(u)}_j(d^*) = \mathbf{\Sigma}_y^{-1}\tilde{\mathbf{\Sigma}}^{(u)}_j(d^*)$, and the predictive variance is thus $c^*_j(d^*) = c_j(d^*, d^*) - \hat{\mathbf{\Sigma}}^{(u)}_j(d^*)^T\tilde{\mathbf{\Sigma}}^{(u)}_j(d^*)$.

For computing the predictive distribution of $j$th interaction functions on multiple test inputs $\mathbf{d}^*_j = [d^*_{1,j}, \ldots, d^*_{N^*_j,j}]^T$, once $\hat{\mathbf{u}}_j = \mathbf{A}_j^T\mathbf{\Sigma}_y^{-1}\mathbf{y}$ is obtained, the direct calculation of the posterior mean involves matrix-vector multiplication $\mathbf{\Sigma}^{(u)}_j(\mathbf{d}^*_j)^T\hat{\mathbf{u}}_j$, which costs $\mathcal{O}(N^*_jN_j)$ if computed directly. This remains computationally intensive for large $N^*_j$, especially during parameter estimation that requires multiple iterations. To reduce computational complexity, we generate an augmented distance vector $\mathbf{d}^{aug,(u)}_j = [(\mathbf{d}^*_j)^T, (\mathbf{d}^{(u)}_j)^T]^T$. We then sort this $(N^*_j + N_j)$-dimensional vector into a non-decreasing sequence: $\mathbf{d}^{aug}_j = [d^{aug}_{1,j}, \ldots, d^{aug}_{N^*_j+N_j,j}]^T$, where $d^{aug}_{t,j} \leqslant d^{aug}_{t',j}$ if $t < t'$. This sorting generates the index set $\{\tilde{g}_t\}_{t=1}^{N^*_j+N_j}$ such that $d^{aug}_{t,j} = d^{aug,(u)}_{\tilde{g}_t,j}$. Next, we define the augmented vector $\hat{\mathbf{u}}^{aug,(u)}_j = [\mathbf{0}^T_{N^*_j}, \hat{\mathbf{u}}^T_j]^T$ of $N^*_j + N_j$ dimensions and rearrange it as $\hat{\mathbf{u}}^{aug}_j$ with $\hat{u}^{aug}_{t,j} = \hat{u}^{aug,(u)}_{\tilde{g}_t,j}$ for $t = 1, \ldots, N^*_j + N_j$. The IKF from Algorithm 1 is then used to compute $\hat{\mathbf{z}}^{aug}_j = \mathbf{\Sigma}^{aug}_j\hat{\mathbf{u}}^{aug}_j$, where $\mathbf{\Sigma}^{aug}_j$ is the covariance matrix of $\mathbf{d}^{aug}_j$. Finally, $\hat{\mathbf{z}}^{aug}_j$ is reordered to the initial order $\hat{\mathbf{z}}^{aug,(u)}_j$ with $\hat{z}^{aug,(u)}_{\tilde{g}_t,j} = \hat{z}^{aug}_{t,j}$, and the predictive mean $\hat{\mathbf{z}}_j(\mathbf{d}^*_j)$ is the first $N^*_j$ entries from $\hat{\mathbf{z}}^{aug,(u)}_{\tilde{g}_t,j}$. This approach reduces computational operations and storage cost to $\mathcal{O}(q_j^3(N^*_j + N_j))$ without approximation.

To compute the predictive variance on multiple test inputs, we employ the IKF to compute the most demanding terms $\mathbf{\Sigma}_y^{-1}\mathbf{A}_j\mathbf{\Sigma}^{(u)}_j(d^*)$ as for predicting on a single test input. Unlike the posterior mean computation, which is required multiple times in parameter estimation, the calculation of the posterior variance only needs to be performed once, making the computation typically feasible after being accelerated by the IKF algorithm. In addition, one may approximate the predictive variance of a test input by the predictive variance on the neighboring grid.

## S5 Application of predicting incomplete lattice for correlated data

Missing values in lattice data are ubiquitous in scientific datasets, such as satellite radar interferograms [1] and temperature measurements [19]. Here, we demonstrate the use of the IKF-CG algorithm to efficiently compute predictions of incomplete lattice data. Let $\mathbf{Z} \in \mathbb{R}^{n_1 \times n_2}$ represent the

unobserved complete lattice data, where the lattice is defined on input variables $\mathbf{s}_1 = [s_{1,1}, \ldots, s_{n_1,1}]$ and $\mathbf{s}_2 = [s_{1,2}, \ldots, s_{n_2,2}]$. Each entry $Z_{i,j}$ corresponds to the value of the function $Z(s_{i,1}, s_{j,2})$ at the input location $(s_{i,1}, s_{j,2})$ on the 2D grid. The lattice is vectorized into an $N$-dimensional vector $\mathbf{z}$ where $\text{vec}(\mathbf{Z}) = \mathbf{z}$ with $\text{vec}(\cdot)$ being the vectorization operator and $N = n_1 \times n_2$. Denote the observed incomplete data as $\mathbf{y}$, consisting of $\tilde{N}$ observations with $\tilde{N} < N$. We model $\mathbf{y}$ as $\mathbf{y} = \mathbf{A}\mathbf{z} + \boldsymbol{\epsilon}$, where $\mathbf{A}$ is a sparse $\tilde{N} \times N$ matrix that maps the latent vector $\mathbf{z}$ to the observed data $\mathbf{y}$. Specifically, $\mathbf{A}$ is formed by removing rows corresponding to missing regions from an $N \times N$ identity matrix, and contains $\tilde{N}$ 1s and $N\tilde{N} - \tilde{N}$ 0s. The Gaussian noise vector follows $\boldsymbol{\epsilon} \sim \mathcal{MN}(\mathbf{0}, \sigma_0^2 \mathbf{I}_{\tilde{N}})$.

For demonstration purposes, we consider $\mathbf{z} \sim \mathcal{MN}(\mathbf{0}, \boldsymbol{\Sigma})$, where $\boldsymbol{\Sigma} = \sigma^2 \mathbf{R}_1 \otimes \mathbf{R}_2$, with $\mathbf{R}_1$ and $\mathbf{R}_2$ being the $n_1 \times n_1$ and $n_2 \times n_2$ correlation matrices of input variables $\mathbf{s}_1$ and $\mathbf{s}_2$ of the lattice, respectively, and $\otimes$ denotes the Kronecker product. Each of $\mathbf{R}_1$ and $\mathbf{R}_2$ is parameterized by a correlation function, such as the Matérn correlation, which enables the use of the IKF for fast matrix-vector multiplication. This framework can be extended to models with semi-separable or non-separable covariances, and distinct mean patterns [10]. After integrating out the latent factors $\mathbf{z}$, the marginal distribution of $\mathbf{y}$ follows

$$\left(\mathbf{y} \mid \boldsymbol{\Sigma}, \sigma_0^2\right) \sim \mathcal{MN}\left(\mathbf{0}, \mathbf{A}\boldsymbol{\Sigma}\mathbf{A}^T + \sigma_0^2 \mathbf{I}_{\tilde{N}}\right).$$

Given the observed data, the posterior distribution of $\mathbf{z}$ is a multivariate normal distribution with mean $\hat{\mathbf{z}}$ given by

$$\hat{\mathbf{z}} = \boldsymbol{\Sigma}\mathbf{A}^T \boldsymbol{\Sigma}_y^{-1} \mathbf{y}, \tag{S16}$$

where $\boldsymbol{\Sigma}_y = \mathbf{A}\boldsymbol{\Sigma}\mathbf{A}^T + \sigma_0^2 \mathbf{I}_{\tilde{N}}$. To calculate the predictive mean, we employ the IKF-CG algorithm. Each iteration of the conjugate gradient algorithm requires computing $\boldsymbol{\Sigma}_y \mathbf{u} = (\mathbf{A}\boldsymbol{\Sigma}\mathbf{A}^T + \sigma_0^2 \mathbf{I}_{\tilde{N}})\mathbf{u}$ for a $\tilde{N}$-dimensional vector $\mathbf{u}$. The most computationally expensive part is computing $\boldsymbol{\Sigma}\mathbf{u} = (\mathbf{R}_1 \otimes \mathbf{R}_2)\mathbf{u} = \text{vec}(\mathbf{R}_2 \mathbf{U} \mathbf{R}_1)$, where $\text{vec}(\mathbf{U}) = \mathbf{u}$. This computation can be accelerated using the IKF algorithm when the correlation matrix is induced by DLM. We first compute $\mathbf{X} = \mathbf{R}_2 \mathbf{U}$ by applying the IKF algorithm column-wise to $\mathbf{U}$, and then compute $\hat{\mathbf{U}} = (\mathbf{R}_1 \mathbf{X}^T)^T$ by again applying the IKF algorithm column-wise. This reduces the computational cost of each matrix-matrix multiplication from $\mathcal{O}(N^2)$ to $\mathcal{O}(q^3 N)$ if we use $q$ latent states for both inputs. Details of parameter estimation are provided in Section S6.

# S6 Parameter estimation

This section discusses the parameter estimation methods for both applications: estimating particle interaction functions (Section 3) and predicting incomplete lattice data (Section S5). In the application described in Section 3, the model parameters include the range parameters $\boldsymbol{\gamma} = (\gamma_1, \ldots, \gamma_J)$, the variance of each latent factor process $\boldsymbol{\sigma}^2 = (\sigma_1^2, \ldots, \sigma_J^2)$, the variance of the noise $\sigma_0^2$, and other physical parameters $\mathbf{r}$, such as the radius of interactions between particles. For computational efficiency, we define $\boldsymbol{\eta} = (\eta_1, \ldots, \eta_J)$ with $\eta_j^2 = \sigma_j^2/\sigma_0^2$ for $j = 1, \ldots, J$ as the ratio of the variance of the $J$ interaction functions to the variance of the noise, and $\sigma_0^2$ can be marginalized out explicitly. This parameterization is preferred over $\sigma_0^2/\sigma_j^2$, because $\sigma_j^2$ could be close to zero if the effect of the $j$th particle interaction is small, thus causing numerical instability. In contrast, the variance $\sigma_0^2$, accounting for measurement noise and model inadequacy, is typically larger than zero, making the parameterization by $\boldsymbol{\eta}$ a preferred choice for our applications. Similarly, for the application in Section S5, we define $\eta = \sigma^2/\sigma_0^2$.

In [11], the authors developed a fast algorithm, which is only applicable for a Gaussian process with an exponential kernel, fixed hyperparameters of covariance functions, and physical parameters.

In this study, we extend the methodology by employing two parameter estimation methods applicable to Gaussian processes with any DLM-induced covariance structure and utilizing the residual bootstrap method for quantifying the uncertainty of parameter estimation. All these approaches can be accelerated using the proposed IKF algorithm.

First, we focus on the cross-validation approach for parameter estimation, where we split the observations into training and hold-out validation sets, denoted as $\mathbf{y}_{train}$ and $\mathbf{y}_{val}$ for $N_{train}$ training and $N_{val}$ validation vectors, respectively. Parameters are estimated by minimizing a loss function, chosen as the mean squared error, during cross-validation:

$$(\hat{\boldsymbol{\eta}}, \hat{\boldsymbol{\gamma}}, \hat{\mathbf{r}}) = \text{argmin}_{(\boldsymbol{\eta},\boldsymbol{\gamma},\mathbf{r})} \left\{ \frac{1}{N_{val}} (\hat{\mathbf{y}}_{val} - \mathbf{y}_{val})^T (\hat{\mathbf{y}}_{val} - \mathbf{y}_{val}) \right\},$$

where for application in Section 3, $\hat{\mathbf{y}}_{val} = \sum_{j=1}^{J} \mathbf{A}_{j,val}\hat{\mathbf{z}}_{j,val}$, with $\hat{\mathbf{z}}_{j,val}$ being the posterior mean of the latent interaction function for cross-validation inputs $\mathbf{d}_j^*$ of size $N_j^*$ and $\mathbf{A}_{j,val}$ being a sparse latent factor loading matrix of dimensions $N_{val} \times N_j^*$, for $j = 1, \dots, J$. For application in Section S5, $\hat{\mathbf{y}}_{val} = \mathbf{A}_{val}\hat{\mathbf{z}}_v$, where $\mathbf{A}_{val}$ is an $N_{val} \times N$ matrix formed by removing rows corresponding to the entries of the training data from an $N \times N$ identity matrix.

Conditioning on other estimated parameters, the maximum likelihood estimate of $\sigma_0^2$ is obtained via $\hat{\sigma}_0^2 = \mathbf{y}^T \mathbf{R}_y^{-1} \mathbf{y} / \tilde{N}$, where $\mathbf{R}_y = \boldsymbol{\Sigma}_y / \sigma_0^2$. The computation of $\mathbf{R}_y^{-1}\mathbf{y}$ can be efficiently handled using the IKF-CG algorithm. The parameters are then transformed to obtain $\hat{\sigma}_j^2 = \hat{\eta}_j^2 \hat{\sigma}_0^2$ and $\hat{\sigma}^2 = \hat{\eta}^2 \hat{\sigma}_0^2$ in applications of Sections 3 and S5, respectively.

Next, we discuss the maximum likelihood estimation, which requires computing the determinant of a large $\tilde{N} \times \tilde{N}$ matrix $\boldsymbol{\Sigma}_y$. This computationally expensive step, requiring $\mathcal{O}(\tilde{N}^3)$ operations in direct computation, can be addressed with a low-rank approximation $\boldsymbol{\Sigma}_a$ of rank $N_a$ for the matrix $\boldsymbol{\Sigma}_0$ [17], with $\boldsymbol{\Sigma}_0 = \sum_{j=1}^{J} \mathbf{A}_j \boldsymbol{\Sigma}_j^{(u)} \mathbf{A}_j^T / \sigma_0^2$ and $\boldsymbol{\Sigma}_0 = \mathbf{A}\boldsymbol{\Sigma}\mathbf{A}^T/\sigma_0^2$ for applications in Sections 3 and S5, respectively. This approach approximates the log-determinant of the covariance matrix by $\log\left|\boldsymbol{\Sigma}_0 + \mathbf{I}_{\tilde{N}}\right| \approx \log\left|\boldsymbol{\Sigma}_a + \mathbf{I}_{N_a}\right|$. The key assumption is that the matrix $\boldsymbol{\Sigma}_0$ has $N_a$ dominant eigenvalues, a sensible assumption for both applications.

To construct $\boldsymbol{\Sigma}_a$, we first set the dimension $N_a$ of the matrix $\boldsymbol{\Sigma}_a$ with $N_a \ll \tilde{N}$ and initialize a $\tilde{N} \times N_a$ matrix $\boldsymbol{\Omega}$ with i.i.d. standard normal entries. Next, we compute $\boldsymbol{\Sigma}_0^{M_0}\boldsymbol{\Omega}$, where $M_0$ is a positive integer. The QR decomposition of $\boldsymbol{\Sigma}_0^{M_0}\boldsymbol{\Omega}$ yields an orthogonal matrix $\mathbf{U} \in \mathbb{R}^{\tilde{N} \times N_a}$, and the low-rank matrix $\boldsymbol{\Sigma}_a$ is defined as $\boldsymbol{\Sigma}_a = \mathbf{U}^T \boldsymbol{\Sigma}_0 \mathbf{U}$. All computations can be accelerated using the IKF method, resulting in a cost of $\mathcal{O}(M_0 \sum_{j=1}^{J} N_j(\log(N_j) + D_y + q_j^3))$ and $O(q^3 M_0 N)$ for applications in Sections 3 and S5, respectively. When the gap between dominant and sub-dominant eigenvalues is large, a small $M_0$ suffices. Figure 3(c) presents the results using $M_0 = 1$, which shows an accurate approximation. Then with the maximum likelihood estimate of $\hat{\sigma}_0^2 = \mathbf{y}^T \mathbf{R}_y^{-1} \mathbf{y} / \tilde{N}$, parameters $(\boldsymbol{\eta}, \boldsymbol{\gamma}, \mathbf{r})$ are estimated by maximizing the logarithm of the marginal likelihood after integrating out the latent factors:

$$(\hat{\boldsymbol{\eta}}, \hat{\boldsymbol{\gamma}}, \hat{\mathbf{r}}) = \underset{(\boldsymbol{\eta},\boldsymbol{\gamma},\mathbf{r})}{\text{argmax}} \left\{ -\frac{1}{2} \log\left|\boldsymbol{\Sigma}_a + \mathbf{I}_{N_a}\right| - \frac{\tilde{N}}{2} \log\left(\mathbf{y}^T \mathbf{R}_y^{-1} \mathbf{y}\right) \right\}.$$

This approximation is as fast as cross-validation, with small approximation errors in our applications, as demonstrated in Fig. 3(c) for a simulated study.

Lastly, we employ residual bootstrap to quantify uncertainty in parameter estimation [4, 18]. This involves computing the posterior mean of the observations $\hat{\mathbf{y}}$ using the predictive interaction function with estimated parameters $(\hat{\boldsymbol{\eta}}, \hat{\boldsymbol{\gamma}}, \hat{\mathbf{r}})$, and calculating residuals $\mathbf{e} = \mathbf{y} - \hat{\mathbf{y}} = [e_1, \dots, e_{\tilde{N}}]^T$. We then generate a new set of $\tilde{N}$ residuals $\mathbf{e}^* = [e_1^*, \dots, e_{\tilde{N}}^*]^T$, such that $\text{pr}(e_i^* = e_{i'}) = 1/\tilde{N}$

| Steps | IKF-CG | CG | Direct computation |
|---|---|---|---|
| Form covariance | / | $O(M\sum_{j=1}^{J} N_j^2)$ | $\mathcal{O}(M\sum_{j=1}^{J} N_j^2)$ |
| Sort inputs | $\mathcal{O}(\sum_{j=1}^{J}(N_j^{all})\log(N_j^{all}))$ | / | / |
| Compute weights | $\mathcal{O}(MS\sum_{j=1}^{J}(D_y+q_j^3)N_j)$ | $O(MS\sum_{j=1}^{J} N_j^2)$ | $\mathcal{O}(M\tilde{N}^3)$ |
| Compute loss | $\mathcal{O}(M\sum_{j=1}^{J}(N_j^{all}))$ | $\mathcal{O}(M\sum_{j=1}^{J} N_j^* N_j)$ | $\mathcal{O}(M\sum_{j=1}^{J} N_j^* N_j)$ |

Table S1: The computational complexity of parameter estimation with $M$ iterations of numerical optimization of the parameters in learning particle interactions with $N_j^{all} = N_j + N_j^*$. The CG and direct computation algorithms involve forming an $N_j \times N_j$ covariance matrix, while the IKF-CG only requires computing the ordered inputs. We assume computing weights $\hat{\mathbf{u}}_j = \mathbf{A}_j^T \mathbf{\Sigma}_y^{-1}\mathbf{y}$ is a separate step with complexity shown in the third row of the table.

for $i' = 1, \ldots, \tilde{N}$. This creates a new set of bootstrap observations via $\mathbf{y}^* = \hat{\mathbf{y}} + \mathbf{e}^*$. Using the same inputs and bootstrap observations, we refit the model to obtain the estimates $\hat{\boldsymbol{\gamma}}^*$, $\hat{\boldsymbol{\eta}}^*$, and $\hat{\mathbf{r}}^*$. Repeating this procedure $B$ times, we obtain confidence intervals by taking the percentiles of these $B$ estimates for each parameter.

# S7 Computational complexity

The primary computational challenge lies in estimating the hyperparameters in the model. Here, we mainly focus on parameter estimation with cross-validation. The computational cost of maximum likelihood estimation is similar. First, we analyze the computational complexity of learning particle interactions in Section 3. Table S1 lists the computational complexity of three different parameter estimation algorithms, namely our IKF-CG method, the conventional conjugate gradient (CG) algorithm, and the direct computation via Cholesky decomposition and forward-backward solver (see Appendix A.4 of [16]). We assume that all algorithms require $M$ iterations for parameter estimation, and in each iteration, the CG and IKF-CG methods require $S$ iterations to compute $\mathbf{\Sigma}_y^{-1}\mathbf{y}$. In our applications, both $M$ and $S$ are around a hundred to ensure the approximation error is a few orders of magnitude smaller than the predictive error (Fig. 3). We will pre-process the particle information and save the results in coarse-grained grids, shown in Fig. S1(a), which only takes $\mathcal{O}(D_y\sum_{\tau=1}^{n_\tau} n_p(\tau)) = \mathcal{O}(\tilde{N})$ operations.

After constructing the neighbors, the cross-validation estimation of the parameters is split into three parts: $\hat{\mathbf{u}} = \mathbf{\Sigma}_y^{-1}\mathbf{y}$, $\hat{\boldsymbol{z}}_j(\mathbf{d}_j^*) = \mathbf{\Sigma}_j^{(u)}(\mathbf{d}_j^*)\mathbf{A}_j^T\hat{\mathbf{u}}$ and $\hat{\mathbf{y}}_{val} = \sum_{j=1}^{J}\mathbf{A}_{val,j}^T\hat{\boldsymbol{z}}_j(\mathbf{d}_j^*)$. To compute $\mathbf{\Sigma}_y^{-1}\mathbf{y}$, we first sort $\mathbf{d}_j^{(u)}$ in a nondecreasing order to obtain the sorted inputs $\mathbf{d}_j$ for each interaction kernel, which requires $\mathcal{O}(\sum_{j=1}^{J} N_j\log(N_j))$ operations. As described in Section S4, for each iteration in the conjugate gradient algorithm, we compute $\mathbf{u}_j^{(u)} = \boldsymbol{A}_j^T\mathbf{u}$ with $\mathbf{u}$ being the current vector for optimization, which requires $\mathcal{O}(D_yN_j)$ operations for $j = 1, \ldots, J$. We then rearrange the vector $\mathbf{u}_j^{(u)}$ to obtain $\mathbf{u}_j$ and use the IKF algorithm to compute $\mathbf{x}_j = \mathbf{\Sigma}_j\mathbf{u}_j$ with a computational cost of $\mathcal{O}(q_j^3N_j)$ for all $j$. After reordering $\mathbf{x}_j$ to get $\mathbf{x}_j^{(u)}$, we compute $\hat{\mathbf{u}}_j = \mathbf{A}_j\mathbf{x}_j^{(u)}$, which again requires $\mathcal{O}(D_yN_j)$ operations. Finally, we calculate $\mathbf{\Sigma}_y\mathbf{u} = \sum_{j=1}^{J}\hat{\mathbf{u}}_j + \sigma_0^2\mathbf{u}$ with $\mathcal{O}(J\tilde{N})$ operations. Typically $N_j \geqslant N$ as the particles contain no less than one neighbor on average. Thus, the total computational operations for $\mathbf{\Sigma}_y^{-1}\mathbf{y}$ amount to $\mathcal{O}(\sum_{j=1}^{J} N_j\log(N_j)) + \mathcal{O}(SD_y\sum_{j=1}^{J} N_j) + \mathcal{O}(S\sum_{j=1}^{J} q_j^3N_j)$, where $S$ is the total number of conjugate gradient iterations. Typically, around 100 iterations are sufficient to provide an accurate estimation in our applications unless the system has extremely

small noise and large correlation, which may make the covariance near singular. Second, computing $\sum_{j=1}^{J} \mathbf{\Sigma}_j^{(u)}(\mathbf{d}_j^*)\mathbf{A}_j^T\hat{\mathbf{u}}$ costs $\mathcal{O}(\sum_{j=1}^{J}(N_j^*+N_j)\log(N_j^*+N_j))+\mathcal{O}(\sum_{j=1}^{J} q_j^3(N_j^*+N_j))$ operations using the IKF algorithm with the augmented covariance matrix and output vector, and the details are discussed in Section S4. Lastly, computing $\sum_{j=1}^{J}\mathbf{A}_{val,j}^T\hat{\mathbf{z}}_j(\mathbf{d}_j^*)$ requires $\mathcal{O}(\sum_{j=1}^{J} D_y N_j^*)$ operations.

In particle interaction applications, $\tilde{N}$ and $N_j$ stand for the number of observations and the number of inputs in the $j$th interaction, respectively, which are typically large in real-world applications, ranging from $10^3$ to $10^6$. The number of validation inputs $N_j^*$ for the $j$th interaction has the same order as $N_j$, and all other quantities listed are relatively small. The number of interactions, $J$, is typically 1 or 2. For modeling interaction functions, Matérn covariances with roughness parameters 0.5 and 2.5 are used, corresponding to $q_j = 1$ and $q_j = 3$, respectively. The dimension of the output vector, $D_y$, is generally no more than 3 in practical scenarios.

The direct computation method requires $\mathcal{O}(M\sum_{j=1}^{J} N_j^2)$ and $\mathcal{O}(M\tilde{N}^3)$ operations for forming the covariance matrix and computing its inversion, respectively, which is prohibitively slow for large dataset. The conjugate gradient algorithm is typically faster than the direct computation method, but still prohibitively expensive to compute $\hat{\mathbf{u}}_j = \mathbf{A}_j^T\mathbf{\Sigma}_y^{-1}\mathbf{y}$ with $MS$ iterations for parameter estimation. The IKF-CG algorithm significantly improves the computational order by removing the cost of forming the $N_j \times N_j$ covariance matrix and computing the weights and loss. It is approximately $N_j$ times faster than the conjugate gradient algorithm for matrix-vector multiplications involving a dense covariance $\mathbf{\Sigma}_j$. The scalability of the IKF-CG algorithm makes it a suitable alternative for fast parameter estimation and predictions.

The computational cost associated with modeling incomplete lattice data using the IKF-CG algorithm is more straightforward. Specifically, parameter estimation for the IKF-CG by cross-validation primarily involves computing the predictive mean in (S16), which requires $\mathcal{O}(MSq^3N)$ operations and $\mathcal{O}(q^3N)$ storage cost, both linear to the size of the covariance matrix. The cost of the IKF-CG algorithm is significantly lower than that of direct computational methods, which require $\mathcal{O}(M\tilde{N}^3)$ for matrix inversion and $\mathcal{O}(\tilde{N}^2)$ for storing the covariance matrix.

# S8 Additional numerical results for estimating interaction functions

## S8.1 Unnormalized Vicsek model

Here we provide additional numerical results for the unnormalized Vicsek model under various scenarios. Figures S2 and S3 present the predictive performance with $\sigma_0^2 = 0.2^2$. Panels (a) and (b) show results for the Matérn kernel with a roughness parameter of 2.5 and the exponential kernel, respectively. As in scenarios with $\sigma_0^2 = 0.1^2$, we observe consistently low NRMSE, with increasing prediction accuracy and decreasing length of the posterior credible intervals, as the number of observations increases.

Figure S4 shows boxplots of the estimated radius parameters for each of the 12 simulated scenarios using the Matérn covariance function with a roughness of 2.5 and exponential covariance. Across all simulations, the estimated radii closely align with the true value $r = 0.5$, and the accuracy of radius estimation improves with larger sample sizes.

To quantify the uncertainty of the estimated radius $\hat{r}$, as well as other parameters, we employ the residual bootstrap method introduced in Section S6. Figure S5 shows the 95% intervals obtained from $B = 100$ bootstrap samples, using the Matérn kernel of roughness parameter 2.5 for two scenarios with $\sigma_0^2 = 0.1^2$ and $\sigma_0^2 = 0.2^2$, where $n_\tau = 5$ and $n_p = 100$ are used for both scenarios. All bootstrap intervals cover the true radius $r$, which indicates a reliable assessment of parameter

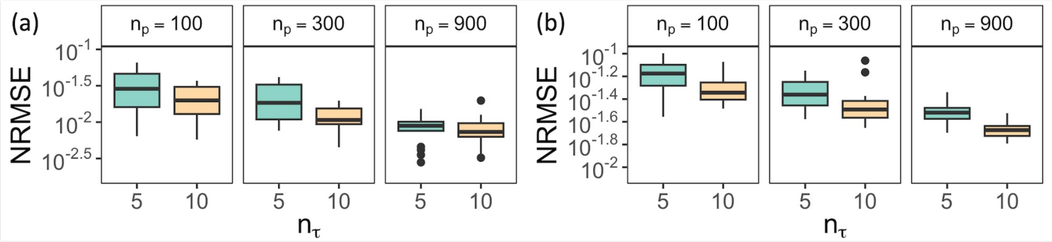


Figure S2: Boxplots of NRMSE (20) for estimating the latent interaction function in the unnormalized Vicsek model with $\sigma_0^2 = 0.2^2$. Results are based on 20 experiments for each scenario, using the Matérn covariance with roughness parameter 2.5 (Panel (a)) and exponential covariance (Panel (b)).

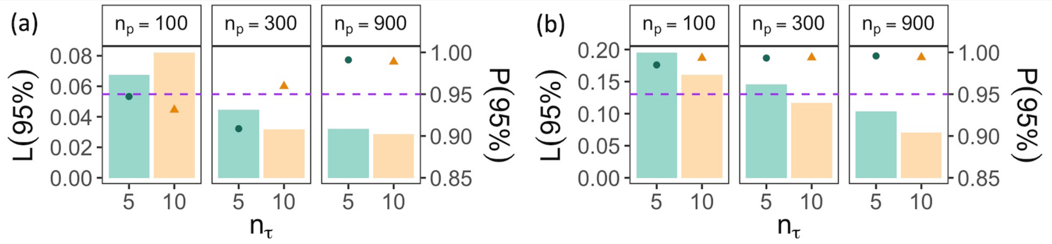


Figure S3: Uncertainty assessment of the predicted interaction function of the unnormalized Vicsek model using the Matérn covariance function with roughness parameter 2.5 (Panel (a)) and the exponential covariance function (Panel (b)), both with $\sigma_0^2 = 0.2^2$. The bars represent the mean length of the 95% posterior credible interval (21) over 20 experiments, and the dots represent the average percentage of test data covered by 95% posterior credible interval (22) across 20 experiments. The purple dashed line at 0.95 indicates the optimal coverage level for the dots.

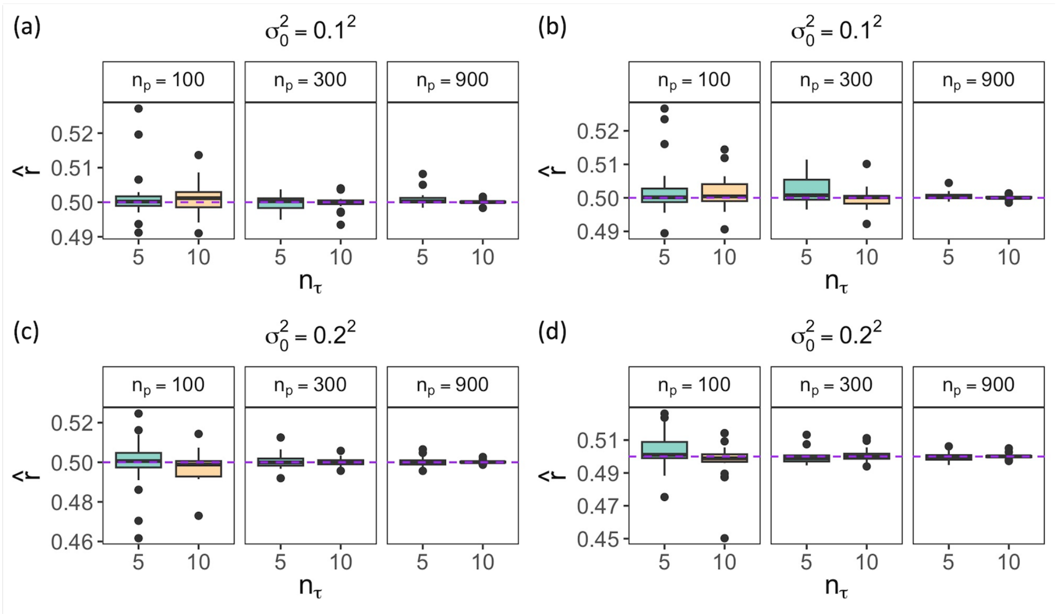


Figure S4: Boxplots of the estimated radius distance $\hat{r}$ in the unnormalized Vicsek model. Panels (a) and (c) use the Matérn covariance with a roughness parameter 2.5 for $\sigma_0^2 = 0.1^2$ and $\sigma_0^2 = 0.2^2$, respectively, while panels (b) and (d) use the exponential covariance for the same noise levels. The purple dashed lines mark the true radius distance $r = 0.5$.

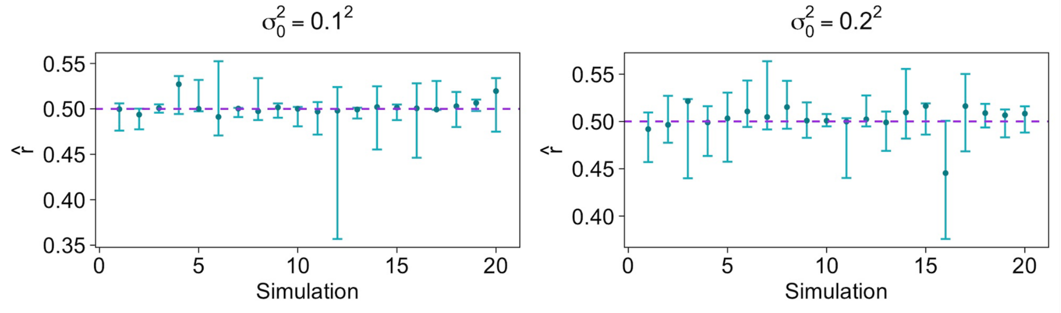


Figure S5: The 95% credible intervals for the estimated interaction radius in the unnormalized Vicsek model, obtained using the Matérn 2.5 covariance and $B = 100$ residual bootstrap samples. Results are based on 20 simulations for $\sigma_0^2 = 0.1^2$ and $\sigma_0^2 = 0.2^2$, with $n_p = 100$ and $n_\tau = 5$. The dots represent the estimated radius $\hat{r}$ from the original data, and the purple dashed lines represent the true radius $r = 0.5$.

uncertainty in these applications.

## S8.2 Modified Vicsek model

| | | First Interaction | | | Second Interaction | | |
|---|---|---|---|---|---|---|---|
| | | NRMSE | $L_1(95\%)$ | $P_1(95\%)$ | NRMSE | $L_2(95\%)$ | $P_2(95\%)$ |
| $n_p = 100$ | $n_\tau = 5$ | $9.9 \times 10^{-3}$ | 0.16 | 98% | $1.6 \times 10^{-1}$ | 0.45 | 93% |
| | $n_\tau = 10$ | $8.9 \times 10^{-3}$ | 0.19 | 94% | $1.0 \times 10^{-1}$ | 0.37 | 94% |
| $n_p = 300$ | $n_\tau = 5$ | $9.7 \times 10^{-3}$ | 0.23 | 98% | $4.8 \times 10^{-2}$ | 0.31 | 97% |
| | $n_\tau = 10$ | $9.2 \times 10^{-3}$ | 0.22 | 96% | $3.5 \times 10^{-2}$ | 0.22 | 96% |
| $n_p = 900$ | $n_\tau = 5$ | $6.2 \times 10^{-3}$ | 0.19 | 100% | $2.5 \times 10^{-2}$ | 0.21 | 99% |
| | $n_\tau = 10$ | $7.3 \times 10^{-3}$ | 0.23 | 99% | $2.0 \times 10^{-2}$ | 0.18 | 99% |

Table S2: The predictive accuracy and uncertainty assessment by (20)-(22) for the modified Vicsek model with $\sigma_0^2 = 0.2^2$ using Matérn covariance function and roughness parameter 2.5.

| | $n_p = 100$ | | $n_p = 300$ | | $n_p = 900$ | |
|---|---|---|---|---|---|---|
| | $n_\tau = 5$ | $n_\tau = 10$ | $n_\tau = 5$ | $n_\tau = 10$ | $n_\tau = 5$ | $n_\tau = 10$ |
| $\sigma_0^2 = 0.1^2$ | $3.5 \times 10^{-3}$ | $2.7 \times 10^{-3}$ | $1.7 \times 10^{-3}$ | $1.1 \times 10^{-3}$ | $4.2 \times 10^{-4}$ | $1.9 \times 10^{-4}$ |
| $\sigma_0^2 = 0.2^2$ | $3.2 \times 10^{-3}$ | $4.0 \times 10^{-3}$ | $1.6 \times 10^{-3}$ | $1.0 \times 10^{-3}$ | $7.9 \times 10^{-4}$ | $3.1 \times 10^{-4}$ |

Table S3: The root mean squared error (RMSE) of the estimated radius for modified Vicsek model using Matérn covariance function with roughness parameter 2.5, computed as $(\sum_{i=1}^{20}(\hat{r}_i - r)^2/20)^{1/2}$ with $\hat{r}_i$ being the estimated radius of the $i$th experiment for each scenario.

The neighbor set in the first term of the modified Vicsek model in (24) is defined as $ne_{i'}(\tau-1) = \{k : ||\mathbf{s}_k(\tau-1) - \mathbf{s}_{i'}(\tau-1)|| < r\}$, with $p_{i'}(\tau-1)$ being the total neighbors in this set. The second term introduces a distance-dependent interaction governed by $f(d_{i',k}(\tau-1)) = -2(5(d_{i',k}(\tau-1) + 0.01))^{-1} - 20d_{i',k}(\tau-1) + 10.8$, where $d_{i',k}(\tau-1) = ||\mathbf{s}_{i'}(\tau-1) - \mathbf{s}_k(\tau-1)||$. This interaction captures repulsion at close distances and attraction at longer distances with the unit vector $\mathbf{e}_{i',k}(\tau-1) = (\mathbf{s}_k(\tau-1) - \mathbf{s}_{i'}(\tau-1))/d_{i',k}(\tau-1)$ specifying the interaction direction. The corresponding neighboring set excludes particle $i'$ itself and is defined as $ne'_{i'}(\tau-1) = \{k : ||\mathbf{s}_k(\tau-1) - \mathbf{s}_{i'}(\tau-1)|| < r \text{ and } i' \neq k\}$, with $p'_{i'}(\tau-1)$ denoting the number of neighbors.

The modified Vicsek model in (24) can be represented as a latent factor model in (13) with two latent interactions. The first interaction is linear, $z_1(d_1) = d_1$, where $d_1 = v_{i',1}(\tau)$ or $d_1 = v_{i',2}(\tau)$, the same as in the unnormalized Vicsek model. The second interaction is nonlinear, $z_2(d_2) = f(d_2)$, where $d_2 = d_{i',k}(\tau-1)$. A common interaction radius $r = 0.5$ is assumed for both interactions.

We first present additional results for Matérn covariance function with a roughness of 2.5 in the modified Vicsek model discussed in Section 4.3, which consists of two types of interaction. Table S2 summarizes the predictive performance with $\sigma_0^2 = 0.2^2$. Consistent with results for $\sigma_0^2 = 0.1^2$, we observe improved performance with an increasing number of observations, especially for the second interaction. Table S3 presents the root mean squared error (RMSE) of the estimated radius. All RMSE values are small, with estimation accuracy improving as the training size increases.

Next, we present the numerical results of latent factor model using an exponential covariance function. The results, presented in Table S4, exhibit similar trends to those obtained by using the Matérn covariance with a roughness parameter of 2.5. Specifically, the NRMSE for the second interaction is larger than that of the first interaction due to fewer observations with small inputs

$\sigma_0^2 = 0.1^2$

| | | First Interaction | | | Second Interaction | | |
|---|---|---|---|---|---|---|---|
| | | NRMSE | $L_1(95\%)$ | $P_1(95\%)$ | NRMSE | $L_2(95\%)$ | $P_2(95\%)$ |
| $n_p = 100$ | $n_\tau = 5$ | $1.1 \times 10^{-1}$ | 0.70 | 88% | $3.6 \times 10^{-1}$ | 1.07 | 92% |
| | $n_\tau = 10$ | $4.9 \times 10^{-2}$ | 0.35 | 94% | $6.7 \times 10^{-2}$ | 0.47 | 98% |
| $n_p = 300$ | $n_\tau = 5$ | $1.2 \times 10^{-1}$ | 0.45 | 84% | $5.3 \times 10^{-2}$ | 0.68 | 98% |
| | $n_\tau = 10$ | $3.1 \times 10^{-2}$ | 0.29 | 92% | $3.3 \times 10^{-2}$ | 0.31 | 99% |
| $n_p = 900$ | $n_\tau = 5$ | $6.6 \times 10^{-2}$ | 0.52 | 91% | $3.0 \times 10^{-2}$ | 0.25 | 98% |
| | $n_\tau = 10$ | $5.4 \times 10^{-2}$ | 0.50 | 91% | $2.5 \times 10^{-2}$ | 0.23 | 99% |

$\sigma_0^2 = 0.2^2$

| | | First Interaction | | | Second Interaction | | |
|---|---|---|---|---|---|---|---|
| | | NRMSE | $L_1(95\%)$ | $P_1(95\%)$ | NRMSE | $L_2(95\%)$ | $P_2(95\%)$ |
| $n_p = 100$ | $n_\tau = 5$ | $6.6 \times 10^{-2}$ | 0.65 | 95% | $1.9 \times 10^{-1}$ | 1.24 | 96% |
| | $n_\tau = 10$ | $4.7 \times 10^{-2}$ | 0.82 | 94% | $1.6 \times 10^{-1}$ | 1.01 | 95% |
| $n_p = 300$ | $n_\tau = 5$ | $8.5 \times 10^{-2}$ | 0.64 | 90% | $8.1 \times 10^{-2}$ | 0.63 | 98% |
| | $n_\tau = 10$ | $8.3 \times 10^{-2}$ | 0.59 | 90% | $5.5 \times 10^{-2}$ | 0.43 | 98% |
| $n_p = 900$ | $n_\tau = 5$ | $7.7 \times 10^{-2}$ | 0.54 | 89% | $4.5 \times 10^{-2}$ | 0.41 | 99% |
| | $n_\tau = 10$ | $4.1 \times 10^{-2}$ | 0.55 | 93% | $3.7 \times 10^{-2}$ | 0.34 | 99% |

Table S4: The prediction results of modified Vicsek model with exponential covariance function.

| | $n_p = 100$ | | $n_p = 300$ | | $n_p = 900$ | |
|---|---|---|---|---|---|---|
| | $n_\tau = 5$ | $n_\tau = 10$ | $n_\tau = 5$ | $n_\tau = 10$ | $n_\tau = 5$ | $n_\tau = 10$ |
| $\sigma_0^2 = 0.1^2$ | $3.1 \times 10^{-3}$ | $1.7 \times 10^{-3}$ | $1.3 \times 10^{-3}$ | $1.3 \times 10^{-3}$ | $3.3 \times 10^{-4}$ | $2.7 \times 10^{-4}$ |
| $\sigma_0^2 = 0.2^2$ | $5.3 \times 10^{-3}$ | $1.9 \times 10^{-3}$ | $2.1 \times 10^{-3}$ | $9.9 \times 10^{-4}$ | $5.1 \times 10^{-4}$ | $2.9 \times 10^{-4}$ |

Table S5: The RMSE of the estimated radius for modified Vicsek model using exponential covariance function.

of the second interaction, which can be resolved by increasing the number of observations. In addition, the length of the 95% posterior credible interval decreases as the number of data points grows, while the coverage proportion remains close to the 95% nominal level. Table S5 displays the RMSE for radius estimation, which exhibits comparable performance to that achieved by using the Matérn covariance with a roughness parameter of 2.5. The accuracy of the estimation improves as we have more observations.

# S9 Numerical results of predicting incomplete lattice data

## S9.1 Evaluation criteria

In this section, we present the results of a simulated study in Section S9.2 and a real data analysis in Section S9.3 to predict incomplete lattices of correlated data. The NRMSE is used to evaluate the predictive performance of the missing regions. Similar to the definition of observation $\mathbf{y}$ in Section S5, the $N - \tilde{N}$ dimensional vector of missing entries is modeled by $\mathbf{y}^{(m)} = \mathbf{A}^{(m)}\mathbf{z} + \boldsymbol{\epsilon}^{(m)}$, where $\mathbf{A}^{(m)} \in \mathbb{R}^{(N-\tilde{N})\times N}$ has $(N - \tilde{N})$ 1s, with all other entries being 0s to map the latent vector to the missing values, and $\boldsymbol{\epsilon}^{(m)}$ is a Gaussian noise vector with variance $\sigma_0^2$. The simulated mean of the missing region is $\mathbf{z}^{(m)} = \mathbf{A}^{(m)}\mathbf{z}$ and the predicted values of the missing region are denoted

as $\hat{\mathbf{z}}^{(m)} = \mathbf{A}^{(m)}\hat{\mathbf{z}}$. The NRMSE in this application is defined as

$$\text{NRMSE} = \left( \frac{\frac{1}{N-\tilde{N}} \sum_{i=1}^{N-\tilde{N}} (\hat{z}_i^{(m)} - z_i^{(m)})^2}{\frac{1}{N} \sum_{i=1}^{N} (\bar{z} - z_i)^2} \right)^{1/2}, \tag{S17}$$

where $\hat{z}_i^{(m)}$, $z_i^{(m)}$, and $z_i$ represent the $i$th entry of $\hat{\mathbf{z}}^{(m)}$, $\mathbf{z}^{(m)}$, and $\mathbf{z}$, respectively, and $\bar{z}$ is the mean of the vector $\mathbf{z}$. Since for real data, the underlying true $\mathbf{z}$ is unknown, the NRMSE in real data analysis in Section S9.3 is computed as in (S17) with $\hat{z}_i^{(m)}$, $z_i^{(m)}$, $z_i$, and $\bar{z}$ replaced by $\hat{y}_i^{(m)}$, $y_i^{(m)}$, $y_i$, and $\bar{y}$, representing the $i$th entry of $\hat{\mathbf{y}}^{(m)}$, $\mathbf{y}^{(m)}$, $\mathbf{y}$ and the average of $[\mathbf{y}^{(m)}, \mathbf{y}]$, respectively.

Our IKF-CG approach is compared with four popular Gaussian process approximation methods, including the Vecchia approximation [20] and Scaled Vecchia approximation (SVecchia) [14], both configured with a model condition size of 90 and a prediction condition size of 150, nearest neighbor Gaussian process (NNGP) [3, 5] with 30 neighbors, and local approximate Gaussian process (laGP) [7, 6] with 70 neighbors. We choose a larger conditioning size of the Vecchia and SVecchia approaches, and more neighbors in NNGP and laGP than the default setting, to improve the precision of the approximation methods, despite the increased computational cost, as shown in Table S6 and Fig. S10. All methods utilize the Matérn kernel with a roughness parameter of 2.5, except for laGP, which only allows the Gaussian kernel in the package.

## S9.2 Branin function

We first employ the Branin function to evaluate the performance of our IKF-CG algorithm in modeling incomplete lattice data [15]. The data are generated using

$$y(s_1, s_2) = \left( s_2 - \frac{5.1}{4\pi^2} s_1^2 + \frac{5}{\pi} s_1 - 6 \right)^2 + 10 \left( 1 - \frac{1}{8\pi} \right) \cos(s_1) + 10 + \epsilon, \tag{S18}$$

where $\epsilon$ is a Gaussian noise with the variance of $\sigma_0^2 = 10^2$. We consider a lattice with dimensions $n_1 = 100$ and $n_2 = 100$ over the domain $(s_{1,i}, s_{2,j}) \in [-5, 10] \times [0, 15]$ for $1 \leqslant i \leqslant n_1, 1 \leqslant j \leqslant n_2$ in (S18). Three scenarios are analyzed, two having 20% missing locations at disks with different centers and one having 20% randomly selected missing locations. In each scenario, we repeat the simulation $E = 20$ times to account for variability from the noise. The observations from the first simulated case of the 20% disk missing scenario are shown in Fig. S6(a), with the underlying mean shown in panel (b). The prediction of the IKF-CG algorithm is plotted in panel (c), which demonstrates a high degree of accuracy.

Figure S7 presents violin plots of the NRMSE distribution for the missing regions in each scenario, comparing IKF-CG with the other four Gaussian process approximation methods, with dots indicating the average NRMSE across all experiments. The results reveal that all methods perform worse with disk-missing data compared to random-missing data, which is expected. Across all scenarios, the IKF-CG consistently achieves the lowest NRMSE values. Specifically, the average NRMSE for the IKF-CG is 0.022, 0.022, and 0.014 for scenarios shown in Fig. S7 (a)-(c), respectively, while the average NRMSE for other methods is at least twice as large. The average computational times for each scenario are provided in Table S6. The Vecchia method is the fastest, while the other four methods have a similar computational time. Overall, the IKF-CG method is more accurate than the alternatives for this example with a similar computational cost.

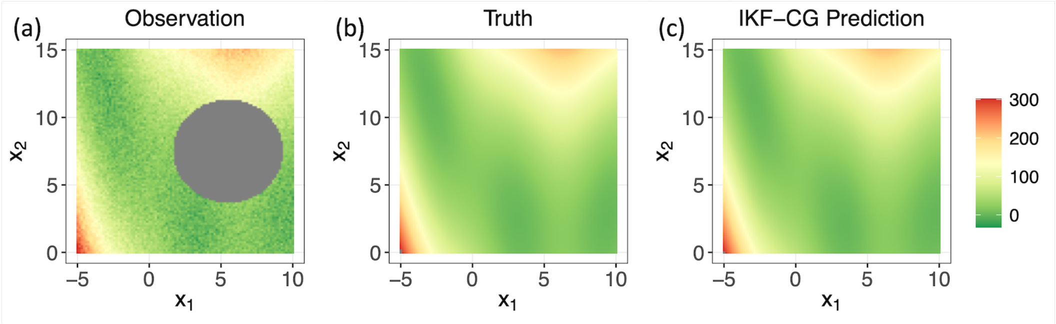


Figure S6: (a) Observed data from a simulation of the Branin function with the first disk missing. (b) Latent mean of the Branin function. (c) Predictions obtained using the IKF-CG algorithm.

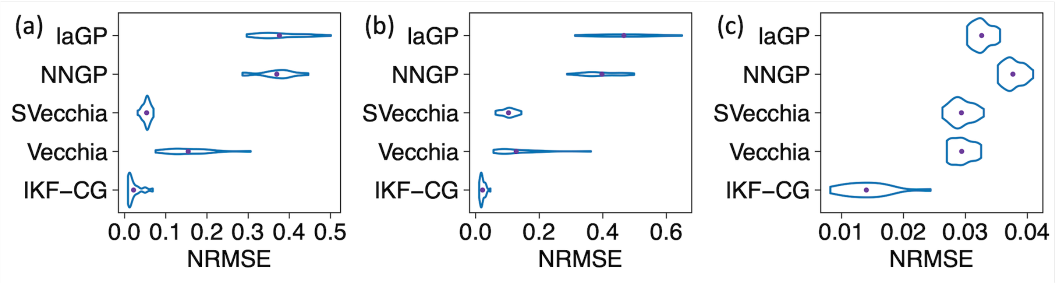


Figure S7: Violin plots illustrating the NRMSE of missing regions for different methods under 20% disk missing with the first center (panel (a)), 20% disk missing with the second center (panel (b)), and 20% random missing (panel (c)). The point on each violin represents the mean NRMSE for each method.

## S9.3 Interferometric synthetic aperture radar interferogram

Interferometric synthetic aperture radar (InSAR) interferograms can measure ground deformation with centimeter-level precision, widely used for understanding geophysical processes and hazard quantification [2, 1]. We test our IKF-CG algorithm for predicting missing values in a COSMO-SkyMed satellite interferogram spanning from October 17, 2011, to May 4, 2012, for Kīlauea Volcano studied in [8]. For demonstration purposes, we investigate two types of missing data on a $200 \times 200$ lattice (disk missing and random missing) across five missing proportions (5%, 10%, 15%, 20%, and 25%).

Figure S8(a) plots the InSAR interferograms with 25% random missing data, while panel (b) shows the complete data without any missing values, and panel (c) presents the predictions obtained using the IKF-CG algorithm. The prediction of IKG-CG shows a high degree of accuracy.

Figures S9(a) and S9(b) illustrate the NRMSE for disk missing and random missing scenarios, respectively. The corresponding run times are provided in Fig. S10, which shows that the computational order of all approaches is similar. Generally, the predictive error is around an order of magnitude smaller for random missing data compared to disk missing data. In Fig. S9(a), the IKF-CG outperforms other methods across most scenarios, especially at higher proportions of missing data (10%, 15%, 20%, and 25%), and it is also the fastest method for these higher proportions shown in Fig. S10. Figure S9(b) reveals that while Vecchia performs slightly better than the IKF-CG for the first four proportions in random missing scenarios, the IKF-CG achieves the lowest NRMSE for the 25% missing scenario. The difference in NRMSE between these two

| | IKF-CG | Vecchia | SVecchia | NNGP | laGP |
|---|---|---|---|---|---|
| Disk1 | 107.1 | 53.2 | 130.6 | 105.2 | 120.4 |
| Disk2 | 108.9 | 52.6 | 142.3 | 105.1 | 120.1 |
| Random | 103.2 | 63.4 | 134.3 | 105.7 | 118.4 |

Table S6: The average computational time in seconds over 20 experiments for estimating the parameters and predicting Branin function.

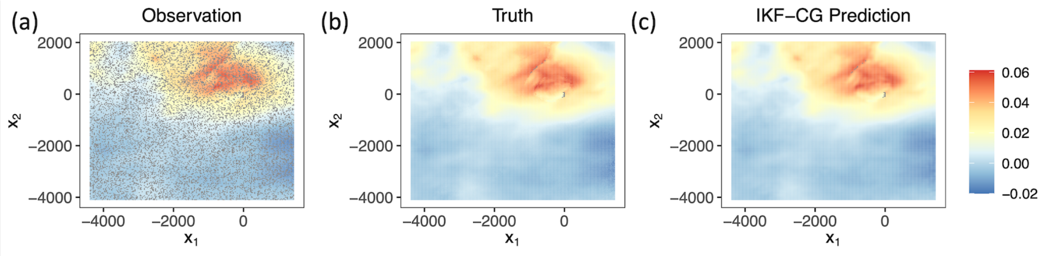


Figure S8: (a) Observed data from interferograms with the 25% random missing. (b) True values of the interferogram data. (c) Predictions obtained using the IKF-CG algorithm.

methods is small. Though predicting missing values in lattice data is not the main application in our study, the results underscore the accuracy and scalability of the IKF-CG algorithm in different applications.

## References


[1] Kyle R Anderson, Ingrid A Johanson, Matthew R Patrick, Mengyang Gu, Paul Segall, Michael P Poland, Emily K Montgomery-Brown, and Asta Miklius. Magma reservoir failure and the onset of caldera collapse at Kīlauea volcano in 2018. *Science*, 366(6470), 2019.

[2] Roland Bürgmann, Paul A Rosen, and Eric J Fielding. Synthetic Aperture Radar Interferometry to Measure Earth's Surface Topography and Its Deformation. *Annual Review of Earth and Planetary Sciences*, 28(1):169–209, may 2000.

[3] Abhirup Datta, Sudipto Banerjee, Andrew O Finley, and Alan E Gelfand. Hierarchical nearest-neighbor Gaussian process models for large geostatistical datasets. *Journal of the American Statistical Association*, 111(514):800–812, 2016.

[4] Anthony Christopher Davison and David Victor Hinkley. *Bootstrap methods and their application*. Number 1. Cambridge university press, 1997.

[5] Andrew O. Finley, Abhirup Datta, and Sudipto Banerjee. spNNGP R Package for Nearest Neighbor Gaussian Process Models. *Journal of Statistical Software*, 103(5):1–40, 2022.

[6] Robert B Gramacy. lagp: large-scale spatial modeling via local approximate Gaussian processes in R. *Journal of Statistical Software*, 72(1):1–46, 2016.

[7] Robert B Gramacy and Daniel W Apley. Local Gaussian process approximation for large computer experiments. *Journal of Computational and Graphical Statistics*, 24(2):561–578, 2015.

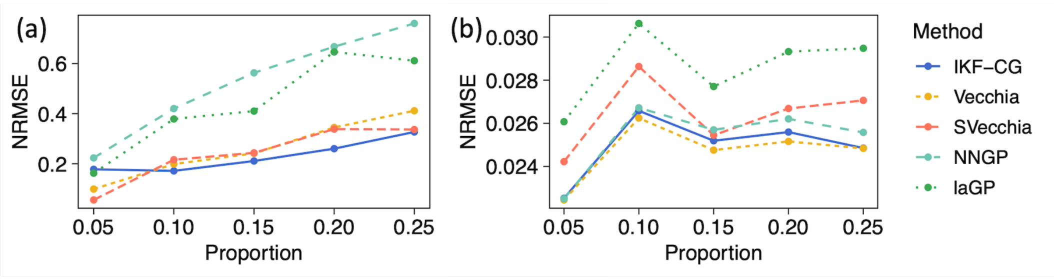


Figure S9: The NRMSE of the missing regions in disk missing (panel (a)) and random missing (panel (b)) scenarios for interferograms.

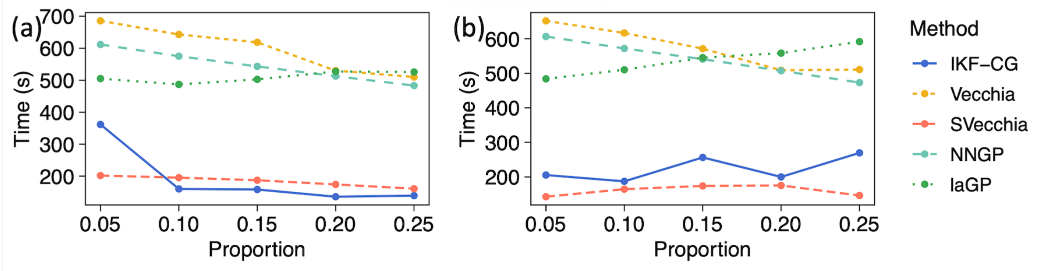


Figure S10: Total computational time for the missing regions in disk missing (panel (a)) and random missing (panel (b)) scenarios for interferograms.


[8] Mengyang Gu, Kyle Anderson, and Erika McPhillips. Calibration of imperfect geophysical models by multiple satellite interferograms with measurement bias. *Technometrics*, 65(4):453–464, 2023.

[9] Mengyang Gu, Xinyi Fang, and Yizi Lin. *FastGaSP: Fast and Exact Computation of Gaussian Stochastic Process*, 2025. R package version 0.6.1.

[10] Mengyang Gu and Hanmo Li. Gaussian Orthogonal Latent Factor Processes for Large Incomplete Matrices of Correlated Data. *Bayesian Analysis*, 17(4):1219 – 1244, 2022.

[11] Mengyang Gu, Xubo Liu, Xinyi Fang, and Sui Tang. Scalable marginalization of correlated latent variables with applications to learning particle interaction kernels. *The New England Journal of Statistics in Data Science*, 1(2):172–186, 2022.

[12] Jouni Hartikainen and Simo Sarkka. Kalman filtering and smoothing solutions to temporal Gaussian process regression models. In *Machine Learning for Signal Processing (MLSP), 2010 IEEE International Workshop on*, pages 379–384. IEEE, 2010.

[13] Magnus R Hestenes and Eduard Stiefel. Methods of conjugate gradients for solving linear systems. *Journal of research of the National Bureau of Standards*, 49(6):409, 1952.

[14] Matthias Katzfuss, Joseph Guinness, and Earl Lawrence. Scaled Vecchia approximation for fast computer-model emulation. *SIAM/ASA Journal on Uncertainty Quantification*, 10(2):537–554, 2022.

[15] Victor Picheny, Tobias Wagner, and David Ginsbourger. A benchmark of kriging-based infill criteria for noisy optimization. *Structural and Multidisciplinary Optimization*, 48(3):607–626, 2013.

[16] Carl Edward Rasmussen. *Gaussian processes for machine learning.* MIT Press, 2006.

[17] Arvind K Saibaba, Alen Alexanderian, and Ilse CF Ipsen. Randomized matrix-free trace and log-determinant estimators. *Numerische Mathematik*, 137(2):353–395, 2017.

[18] Jun Shao and Dongsheng Tu. *The jackknife and bootstrap.* Springer Science & Business Media, 2012.

[19] Jonathan R Stroud, Michael L Stein, and Shaun Lysen. Bayesian and maximum likelihood estimation for Gaussian processes on an incomplete lattice. *Journal of computational and Graphical Statistics*, 26(1):108–120, 2017.

[20] Aldo V Vecchia. Estimation and model identification for continuous spatial processes. *Journal of the Royal Statistical Society: Series B (Methodological)*, 50(2):297–312, 1988.
